# Supplementary material for: Stellar populations of the globular cluster NGC 5053 investigated using AstroSat-Ultra Violet Imaging Telescope
Source: arXiv:2205.13839 ancillary file (2022-06-13)
Supplement: Supplementary file 1 [file ngc5053_Supplementary_figure.pdf]

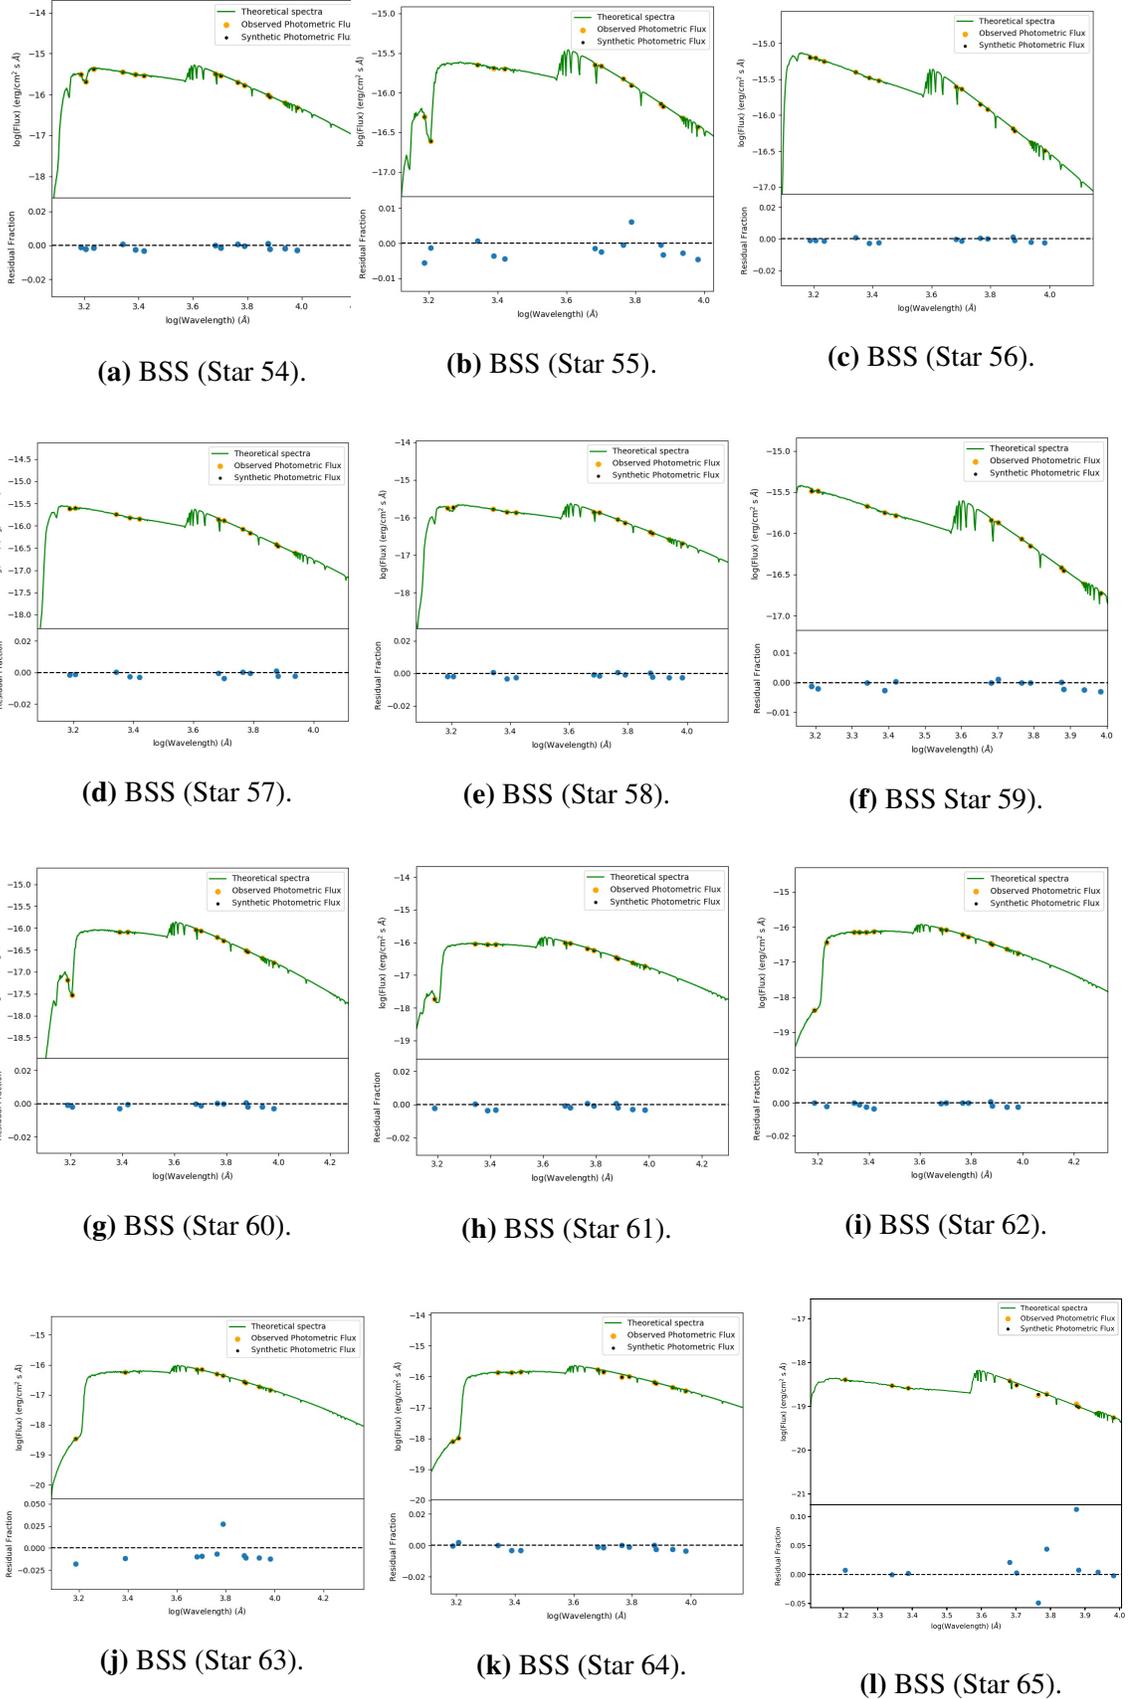

**Figure 1.1:** Spectral energy distributions of the BSS population in NGC 5053. The Star number indicated in the parenthesis represents the serial number of the BSS star/candidate as given in the catalog.

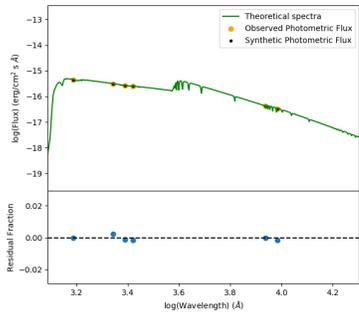

(m) BSS (Star 67).

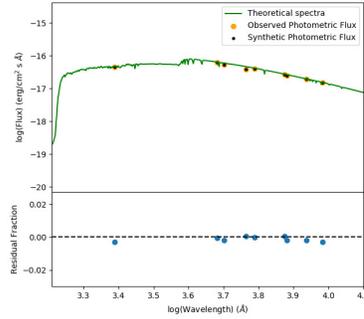

(n) BSS (Star 69).

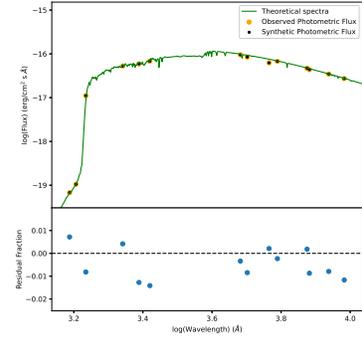

(o) BSSc (Star 70).

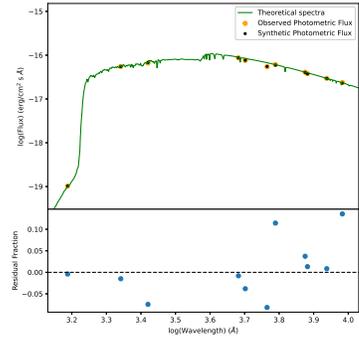

(p) BSSc (Star 71).

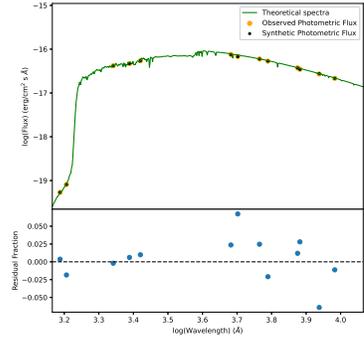

(q) BSSc (Star 72).

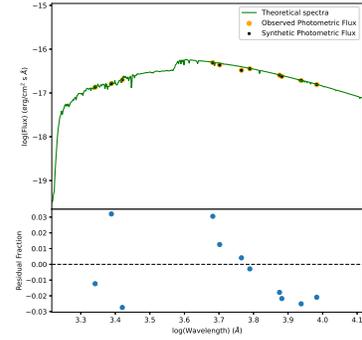

(r) BSSc (Star 73).

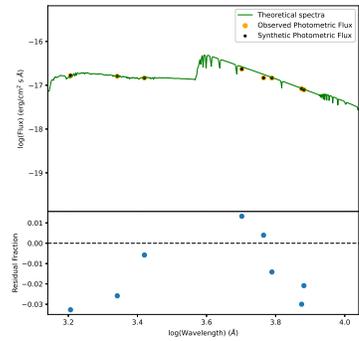

(s) BSSc (Star 74).

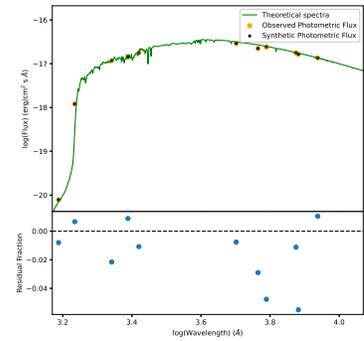

(t) BSSc (Star 75).

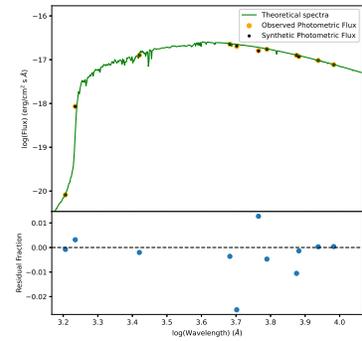

(u) BSSc (Star 76).

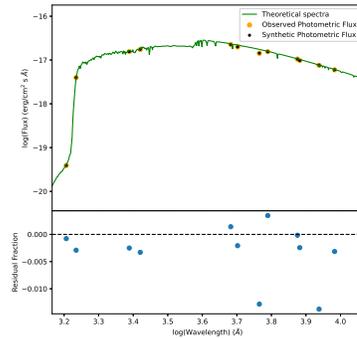

(v) BSSc (Star 77).

**Figure 1.1:** Spectral energy distributions of the BSS population in NGC 5053. The Star number indicated in the parenthesis represents the serial number of the BSS star/candidate as given in the catalog.
